# Supplementary material for: EulerFormer: Sequential User Behavior Modeling with Complex Vector Attention
Source: arXiv:2403.17729 source file (2024-04-04)
Supplement: Supplementary file 1 [file sec-appendix.tex]

\section{Appendix}\label{sec:appendix}
% \section{Appendix: ALIGN WITH HIGH ORDER METHODS}\label{sec:appendix}
The demonstration of DAGFM-inner and DAGFM-kernel of polynomial approximation with CIN and CrossNet respectively.

\noindent\textbf{Notations.}
Let multi-index $\bm \alpha = [\alpha_1,...,\alpha_d] \in \mathbb{N}^d$ and $|\bm \alpha|=\sum_{i=1}^d \alpha_i$. 
$\bm C_a^b=\{ \bm y \in \{1,...,a\}^b | \forall{i<j},y_i \leq y_j \}$ and  $\bm T_a^b = \{ \bm y \in \{1,...,a\}^b | \forall i < j , y_i > y_j \}$

\noindent\textbf{DAGFM-inner v.s. CIN.}
We assume that the multiplication operation is vector-wise and a superscript is used to denote
the vector operation such as $\bm x_i \bm x_j = \bm x_i \odot \bm x_j$ , $\bm x_i^2 = \bm x_i \odot \bm x_i$. 
As it is discussed in Section 3.1.3, $\bm h_i^{t}$ in DP denotes the sum of all $t$-order feature interactions suffixed with $\bm e_{i}$.
 i.e.,
 \begin{equation}
  \bm h_i^{t} = \sum_{j \in \bm C_{i}^{t-1} } {\bm e_{j_1}  \bm e_{j_2}  ...  \bm e_{j_{t-1}}  \bm e_i}
\end{equation}

$\bm h_i^{t}$ in DP can be regarded as the simplified expression of the node state vector when omitting the interacting weight. We degenerate the edge weight of DAGFM-inner from vector to scalar, \ie $\bm w_{i,j}^t = w_{i,j}^t \bm 1$.
And we can get the weight of $\bm e_{j_1}  \bm e_{j_2}  ...  \bm e_{j_{t-1}}  \bm e_i$ through the propagation path and thus we have:
\begin{equation}
  \bm h_i^{t} = \sum_{\bm j \in \bm C_{i}^{t-1} } (w_{j_1,j_2}^1 w_{j_2,j_3}^2 ...  w_{j_{t-1},i}^{t-1}){\bm e_{j_1}  \bm e_{j_2}  ...  \bm e_{j_{t-1}}  \bm e_i}
\end{equation}

Therefore, DAGFM-inner with depth $l$ reproduces interaction polynomials in the following class 
: 
\begin{equation}
  \Big\{\sum_{\bm \alpha}{\phi_{\bm \alpha}\bm e_1^{\alpha_1} \bm e_2^{\alpha_2}  ...  \bm e_m^{\alpha_m}} \Big|  2 \leq |\bm \alpha| \leq l+1 \Big\},
  \label{eq:innerg}
\end{equation}
where $\phi_{\bm \alpha} ={
    \prod_{i = 1}^{|\bm \alpha|-1}{w_{S_{\bm \alpha}[i],S_{\bm \alpha}[i+1]}^{i}}}$
is weight of corresponding feature interaction,
$\bm S_{\bm \alpha} = \bigcup_{i=1}^{m}{\{\underbrace{i, ... ,i}_{\bm \alpha_i times}
\Big| \alpha_i \neq 0 \}}$ and $\bm S_{\bm \alpha}[i]$ is the $i$-th element of $\bm S_{\bm \alpha}$.
Specially, the $k$-layer CIN's formula is given by:
\begin{equation}
  {\Big\{\sum_{\bm \alpha}\phi_{\bm \alpha}\bm e_1^{\alpha_1}\bm e_2^{\alpha_2}...\bm e_m^{\alpha_m}} \Big|2\leq|\bm \alpha|\leq k+1\Big\},
  \label{eq:cinc}
\end{equation}
where $\phi_{\bm \alpha}$ can be estimated as:
$
  \hat{\phi}_{\bm \alpha}=\sum_{i=1}^m \sum_{j=1}^m \sum_{\bm B \in \bm P_{\bm \alpha}} \prod_{t=2}^{|\bm \alpha|}{W_{i,B_t}^{t,j}}$
and $\bm P_{\bm \alpha}$ is the set of all permutations of the ${\bm S_{\bm \alpha}}$.

Therefore, DAGFM-inner has a similar formula to CIN (see Eq. \ref{eq:innerg} and Eq. \ref{eq:cinc}). 

\noindent\textbf{DAGFM-kernel v.s. CrossNet.}
Similar to DAGFM-inner, the output of $l$-layer 
DAGFM-kernel
creates the feature interactions up to order $l+1$. 
Their $p$-order interaction is given by:
\begin{equation}
  \sum_{j \in \bm I_p}{((\bm e_{j_1}\bm w_{j_1,j_2}^{1}) \odot ... \odot \bm e_{j_{p-1}} \bm w_{j_{p-1},j_{p}}^{p-1})\odot \bm e_{j_p}},
  \label{eq:gfmker}
\end{equation}
where $\bm I_p = \Big\{\bm S_{\bm \alpha} \Big| |\bm \alpha|=p \Big\}$ and $j_k$ is the $k$-th element of $j$.
Similarly, the $p$-order feature interactions of CrossNet is given by:
\begin{equation}
\sum_{\bm i \in \bm P_{\bm \alpha}}\sum_{\bm j \in \bm T_{p}^{p-1}}\bm e_{i_1} \odot (\bm W_{i_1,i_2}^{j_1}
\bm e_{i_2}\odot...\odot(\bm W_{i_k,i_{k+1}}^{j_{p-1}}\bm e_{i_p})),
\label{eq:cross}
\end{equation}
where $|\bm \alpha| = p$. We can see that DAGFM-kernel has a similar formula to CrossNet (see Eq. \ref{eq:gfmker} and Eq. \ref{eq:cross}).
